# Supplementary material for: Process Extraction from Text: Benchmarking the State of the Art and Paving the Way for Future Challenges
Source: arXiv:2110.03754 source file (2023-10-25)
Supplement: Supplementary file 1 [file appendix.tex]

\section{Appendices}
\label{sec:appendices}
        We report below an anonymized excerpt of the procedural section of a Standard Operative Procedure (SOP) adopted in a company. 
        The text of the SOP is reported anonymized and simplified with abbreviations resolved and punctuation fixed.
        
        SOPs documents differ greatly to those released in~\citep{Friedrich11}.
        In particular, each document of the data set is made of almost ten pages each with many sections, typically composed by very long sentences with an extensive use of topic specific terms and abbreviations.
        These documents vary greatly in the writing style adopted because they were written by different authors along the years.
        Indeed, in some of them, the procedure description is written without bullet-lists and have longer sentences.
        Other cases exhibit the opposite pattern.
        
        The second paragraph reports a full text of a process description proposed in~\citep{Friedrich11}.
        The reader can easily notice the great difference between the two texts.
        Indeed, different from SOPs, the samples proposed in~\citep{Friedrich11} result to be more easier to analyse because they are almost free of uninformative text and because process elements are easy to extract by mean of patterns.
        
        \subsection{Excerpt of a Standard Operative Procedure. Access for new Users.}
        \label{sssec:qa-excerptSOP}
            Every User has an unique user name, which is the same for all three environments.
            The password is different for every environments and every User is responsible to keep credentials as appropriate and to not share them with other Users or people.
            The password shall be changed periodically, upon prompt from the system, before the expiry date.
            Third Party Provider staff and other consultant(s) may gain access the database only after specific training performed by:
             - an XIS trainer, who will release a training certificate or
             - a ABC Company experienced Standard User who shall train the new User on the job: certificate is released by the ABC Company experienced Standard User after the User has successfully processed at least 10 case reports in the Sandbox.
            When the training is completed, upon Qualified Person for approval, a ABC Company Administrator User shall request to DEF company global access for the individual user (see par. X.xx), assigning specific roles according to the activities to be performed by the User.
            Access is released by DEF company to the individual User who receives username and password directly from the Help-desk.
            Users shall have access to the system - User Manuals available on the knowledge portal, containing a detailed description of how the system works and how to perform all activities for case processing.
            
        \subsection{A sample of the data set used in~\citep{Friedrich11}}
        \label{sssec:qa-textfriedrich}
            The MPON sents the dismissal to the MPOO.
            The MPOO reviews the dismissal.
            The MPOO opposes the dismissal of MPON or the MPOO confirms the dismissal of the MPON.
